# Supplementary material for: Atypical antiferromagnetic ordering in single crystalline quasi-2D honeycomb magnet YbI$_3$
Source: arXiv:2407.01982 source file (2024-07-02)
Supplement: Supplementary file 1 [file YbI3-Supplemental-Material.pdf]

# Supplemental Material: Atypical antiferromagnetic ordering in single crystalline quasi-2D honeycomb magnet $YbI_3$


Nashra Pistawala,[1] Luminita Harnagea,[2] Sitaram Ramakrishnan,[1,2]
Priyanshi Tiwari,[3] Rajeev Rawat,[3] and Surjeet Singh[1,*]

[1]*Department of Physics, Indian Institute of Science Education and Research, Pune, Maharashtra-411008, India*

[2]*I-HUB Quantum Technology Foundation, Indian Institute of Science Education and Research, Pune-411008*

[3]*UGC-DAE Consortium for Scientific Research, University Campus, Khandwa Road, Indore 452 001*

### A. Crystal growth

$YbI_3$ single crystals were grown using physical vapor transport reaction using three different temperature profiles in order to obtain high-quality crystals. Initially, the crystal growth ampoule was kept in a temperature gradient furnace with source and sink temperatures at 750 °C and 650 °C, respectively, for 20 days, later the temperature was lowered to room temperature at a rate 100 °C/hr. The crystals were of high quality but smaller in size. In the next growth attempt, the ampoule was kept at similar temperatures for 24 hours and later gradually cooled at a rate of 0.3 °C/hr. The slow cooling helped to grow cm-sized large single crystals. Attempts to grow crystals at high temperatures were unsuccessful and led to very few mm-sized crystals in the reaction ampoule. The different growth conditions adapted to obtain high-quality single crystals of $YbI_3$ are summarized in Table S1. The crystals obtained from the growth attempt labeled as 2 are the largest, and hence, these crystals are used in all further investigations.

TABLE S1. Summary of various parameters used during the crystal growth attempts: Source temperature ($T_{source}$ ), sink temperature($T_{sink}$), Dwell time, Rate of cooling, and total duration of the crystal growth experiment needed to obtain high-quality single crystals.

| Growth attempt | $T_{source}$ | $T_{sink}$ | Dwell time | Rate of cooling | Duration | Conclusion |
|---|---|---|---|---|---|---|
| 1 | 750 °C | 650 °C | 20 days | 100 °C/hr below 650 °C | 30 days | Many small crystals of typical Size ranging from 3 - 4 mm lateral dimension |
| 2* | 750 °C | 650 °C | 24 hours | 0.3 °C/hr($T_{source}$ = 750 °C to 600 °C) | 30 days | large crystals of Size nearly 10 mm lateral dimension |
| 3 | 1050 °C | 1000 °C | 24 hours | 0.3 °C/hr($T_{source}$ = 1050 °C to 900 °C) | 30 days | very few small crystals of size 1 mm lateral dimension |

∗The optimal thermodynamic conditions for obtaining centimeter-sized crystals have been identified, and crystals from this batch are being used for further analysis in this study.

### B. Chemical composition of $YbI_3$

The Chemical composition was checked on a crystal specimen shown in the Fig. S1(a). The EDX spectra were collected at 15 - 20 different areas marked with yellow rectangles

* email:surjeet.singh@iiserpune.ac.in

on the specimen in order to confirm the homogeneity. The atomic % for Yb and I and their corresponding Composition is shown in Table S2. The data was corrected using ZFA method. The error bar in the measurement was approximately 4 - 5 atomic %. The sample begins to crack once it is exposed to the ambient atmosphere. During loading into the sample chamber, the specimen was exposed to the atmosphere for a few seconds, resulting in slight cracking in the few parts of the sample as seen in the SEM image.

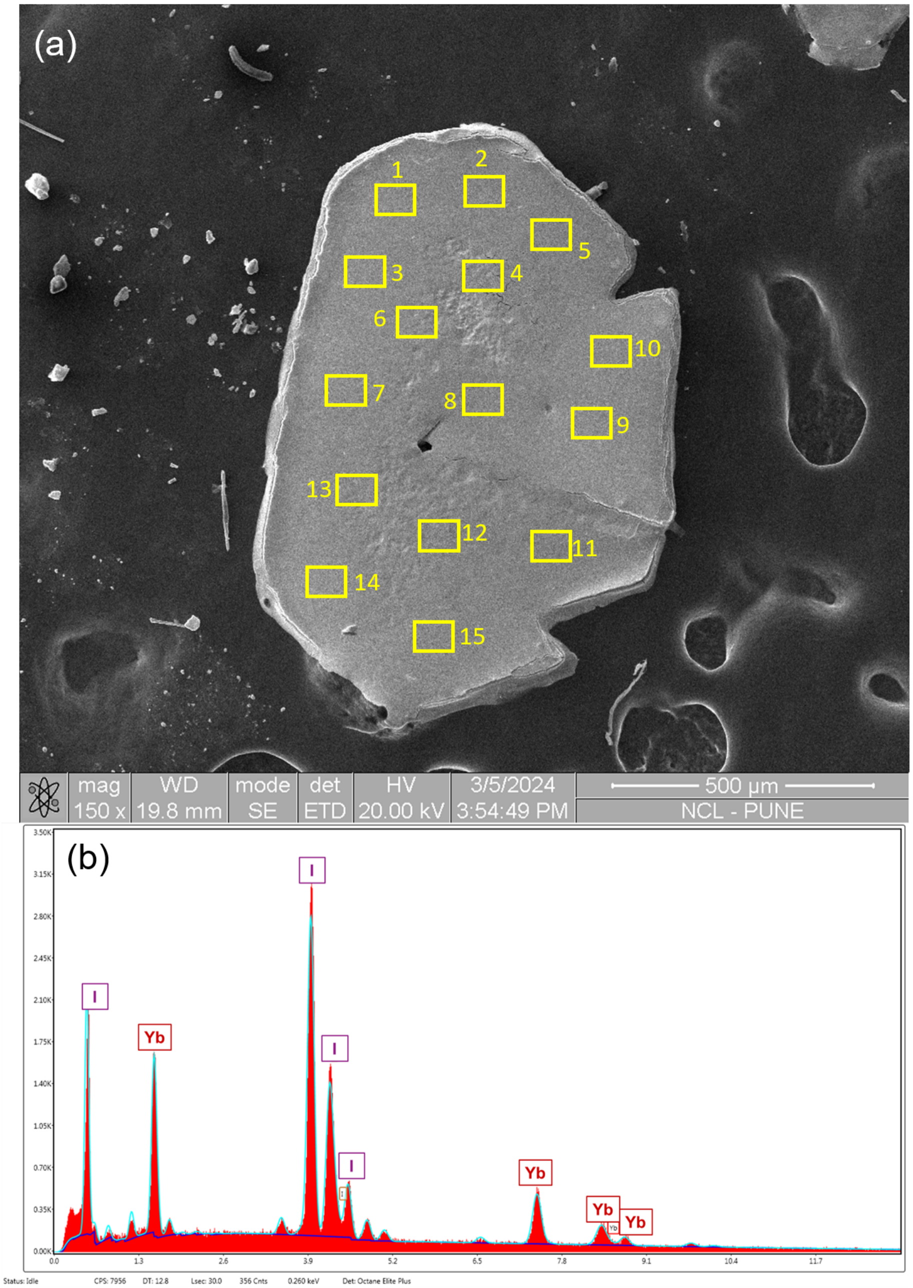


Fig. S1. EDX spectra taken at 15 different areas to show the homogeneity of the single crystal. (a) The scanning electron microscope image of $YbI_3$ crystal specimen taken using Secondary electron (SE) mode. The yellow rectangles marked on the images are different areas on which EDX spectra was collected. One such spectrum is shown in the (b).

TABLE S2. The composition of Yb and iodine at 15 different areas of the single crystal shows the homogeneity of the crystal specimen.

| Area | Yb (atomic %) | I (atomic %) | Yb (composition) | I (composition) |
|---|---|---|---|---|
| 1 | 23.52 | 76.48 | 0.9408 | 3.0592 |
| 2 | 24.76 | 75.24 | 0.9904 | 3.0096 |
| 3 | 23.34 | 76.66 | 0.9336 | 3.0664 |
| 4 | 23.4 | 76.6 | 0.936 | 3.064 |
| 5 | 23.33 | 76.67 | 0.9332 | 3.0668 |
| 6 | 23.4 | 76.6 | 0.936 | 3.064 |
| 7 | 21.85 | 78.15 | 0.874 | 3.126 |
| 8 | 23.36 | 76.64 | 0.9344 | 3.0656 |
| 9 | 22.88 | 77.12 | 0.9152 | 3.0848 |
| 10 | 23.46 | 76.54 | 0.9384 | 3.0616 |
| 11 | 24.4 | 75.6 | 0.976 | 3.024 |
| 12 | 24.11 | 75.89 | 0.9644 | 3.0356 |
| 13 | 23.25 | 76.75 | 0.93 | 3.07 |
| 14 | 22.51 | 77.49 | 0.9004 | 3.0996 |
| 15 | 23.62 | 76.38 | 0.9448 | 3.0552 |

## C. Raman Spectra of $YbI_3$

The comparison between the Raman modes for $YbI_3$ and $Dy_3$ is tabulated in Table. S3. The symmetry of modes in the $D_{3d}$ point group according to the group theory is also shown for the reference.

TABLE S3. Experimental Peak position for $YbI_3$ and $DyI_3$ at room temperature

| Label | Positions($cm^{-1}$) $YbI_3$ (This work) | Positions($cm^{-1}$) $DyI_3$ [1] | Mode($D_{3d}$) |
|---|---|---|---|
| $P_1$ | 38.41 | 39 | $E_g$ |
| $P_2$ | 56.42 | 55 | $A_{1g}$ |
| $P_3$ | 69.43 | 71 | $E_g$ |
| $P_4$ | 94.04 | 94 | $E_g$ |
| $P_5$ | 118.56 | 120 | $A_{1g}$ |
| $P_6$ | 142.51 | 146 | $E_g$ |
| $M_1$ | 61.63 | - | - |
| $M_2$ | 74.35 | - | - |
| $M_3$ | 114.10 | - | - |
| $M_4$ | 137.53 | 139 | - |

## D. Single crystal x-ray diffraction reciprocal space images for $YbI_3$

The single crystal x-ray diffraction on several single crystal specimens confirms the $R\bar{3}$ symmetry of the structure. To further substantiate this point, we plotted the reciprocal space cuts along (0 k l) direction for two different temperatures 250 K and 150 K as shown in Fig. S2(a,b). The two-dimensional plot for the rectangle marked in Fig. S2(a,b) is shown in Fig. S2(c,d) indicating the (0 k l) reflections, which satisfies the general condition for trigonal symmetry, that is, $-h + K + l = 3n$. Hence, the $R\bar{3}$ symmetry of $YbI_3$ was confirmed at room temperature down to 150 K.

The atomic coordinates along with the anisotropic displacement parameters is shown in Table S4

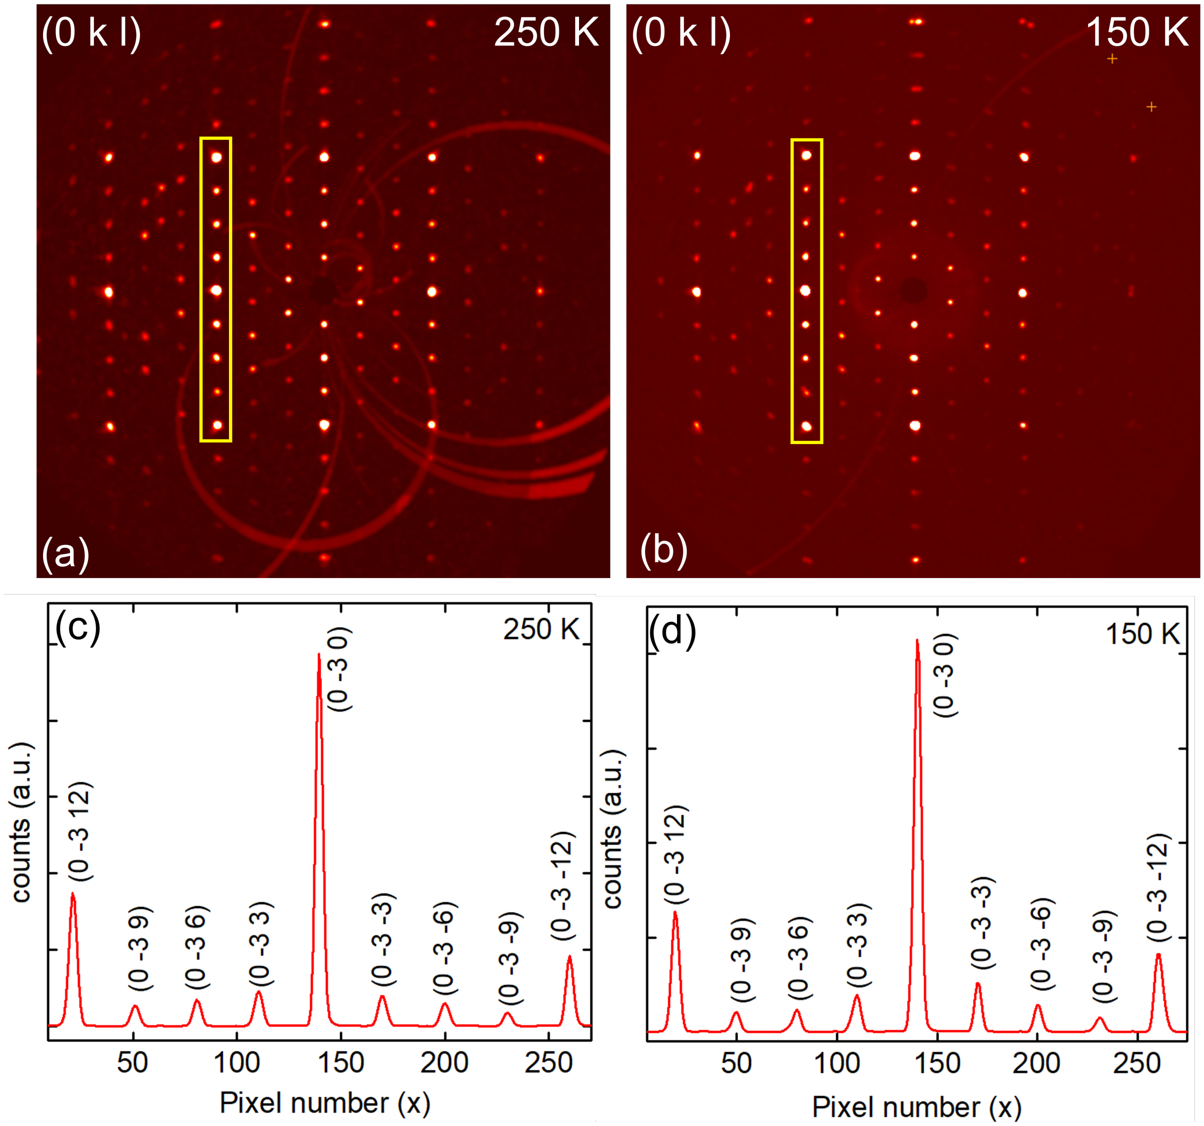


Fig. S2. Reconstructed plot of reciprocal space along (0 k l) direction.(a) 250 K. (b) 150 K. Two-dimensional plot of ( 0 k l) reflections marked as a rectangle in (a) and (b). The x-axis indicates the x-coordinate (position) of the spots in units of detector pixel, and y-axis indicates the intensity of the spots

TABLE S4. Atomic Coordinates x, y, z and anisotropic displacement parameters(ADPs) of single crystal at 250 K in Å$^2$ . Unique reflections (obs/all) = 561/728, criterion of observability: $I > 3\sigma(I)$, $R_F = 0.0556$, No. of refined paramateres = 14, Refinement method used: least-squares on F, Space group: $R\bar{3}$.

| Atoms | Wyck | x | y | z | $U_{11}$ | $U_{22}$ | $U_{33}$ | $U_{12}$ | $U_{13}$ | $U_{23}$ | $U_{iso}^{eqi}$ |
|---|---|---|---|---|---|---|---|---|---|---|---|
| Yb | 6c | 0 | 0 | 0.3337 | 0.0151 | 0.0151 | 0.0244 | 0.0075 | 0 | 0 | 0.0182 |
| I | 18f | 0.3229 | 0.3341 | 0.4165 | 0.0239 | 0.0185 | 0.0242 | 0.0092 | -0.0059 | -0.0003 | 0.0228 |

[1] A. Chrissanthopoulos, G. D. Zissi, and G. N. Papatheodorou, Zeitschrift für Naturforschung A **60**, 739 (2005).
